# Supplementary material for: STYLER: Style Factor Modeling with Rapidity and Robustness via Speech Decomposition for Expressive and Controllable Neural Text to Speech
Source: arXiv:2103.09474 source file (2021-06-25)
Supplement: Supplementary file 1 [file table.tex]

\begin{table}[h]
    \centering
    \caption{Configuration of encoders}
    \begin{threeparttable}
        \resizebox{0.45\textwidth}{!}{
        \begin{tabular}{l|cccc}
            \hline\hline
            \multicolumn{1}{c}{} & Duration & Pitch & Energy & Noise  \\
            \hline
            \ \textbf{Conv Layers} & 3 & 3 & 3 & 3 \\
            \hline
            \ \textbf{Conv Dim} & 256 & 320 & 320 & 256 \\
            \hline
            \ \textbf{Norm Groups} & 16 & 20 & 20 & 16 \\
            \hline
            \ \textbf{BLSTM Layers} & 2 & 2 & 2 & 2  \\
            \hline
            \ \textbf{BLSTM Dim} & 64 & 64 & 64 & 64  \\
            \hline
        \end{tabular}}
    \end{threeparttable}
    \label{tab:encoder}
\end{table}
